# Supplementary material for: Can You See Me Now? A Measurement Study of Zoom, Webex, and Meet
Source: arXiv:2109.13113 source file (2021-09-27)
Supplement: Supplementary file 1 [file appendix.tex]

\appendix
%%%%%%%%%%%%%%%%%%%%%%%%%%%%%%%%%%%%%%%%%%%%%
\section{Appendix Title}
\label{sec:appendix}
%%%%%%%%%%%%%%%%%%%%%%%%%%%%%%%%%%%%%%%%%%%
TODO
